# Supplementary material for: Does the Whole Exceed its Parts? The Effect of AI Explanations on Complementary Team Performance
Source: arXiv:2006.14779 source file (2021-01-12)
Supplement: Supplementary file 1 [file appendix.tex]

\section{Appendix}

\subsection{Choosing a Classification Model \& Explanation Method}
\label{subsec:explainer_select}

While various studies have been conducted to compare explanations from different aspects (\eg.~\cite{nguyen2018comparing, Hase2020EvaluatingEA}), there has yet to be a clear conclusion on which models/explainers perform the best.
For our studies, we wished to select a model that offered both credible predictions and explanations. 
So, we compared three approaches, which broadly covered existing NLP models for generating explanations along with predictions~\cite{nguyen2018comparing, lipton-icmlwhi16}: an intelligible model ({\em Logistic Regression} classifier), a encoder-decoder {\em rationale generator} (Lei \etal~\cite{lei2016rationalizing}), and a recent contextual embedding-based model ({\em RoBERTa} with linear classification layer). While the first two models inherently generate explanations by providing access to weight vectors which represent salience of input words for predictions, the third method is a black-box and requires using a {\em post-hoc explainer} to generate explanations. We tried three existing post-hoc explainers to explain the RoBERTa model: {\em LIME} trains a new intelligible model to provide a local approximation of a model's behavior\cite{ribeiro-kdd16}, {\em SimpleGrad} computes gradients with respect to input, and {\em IntergratedGrad} uses an approach that aggregates multiple gradients~\cite{sundararajan2017axiomatic}.\footnote{Implementation: For logistic regression we used scikit-learn, for the rational generator we used re-implementaion by \cite{deyoung2019eraser}, and, we used AllenNLP's demo code for classification using RoBERTa \url{https://demo.allennlp.org/sentiment-analysis}. For the post-hoc explainers, we used LIME's original implementation \cite{ribeiro-kdd16} and AllenNLP Interpret~\cite{wallace2019allennlp} for gradient-based explainers.}

\begin{figure}[t]
 \centering
 \includegraphics[width=1\columnwidth]{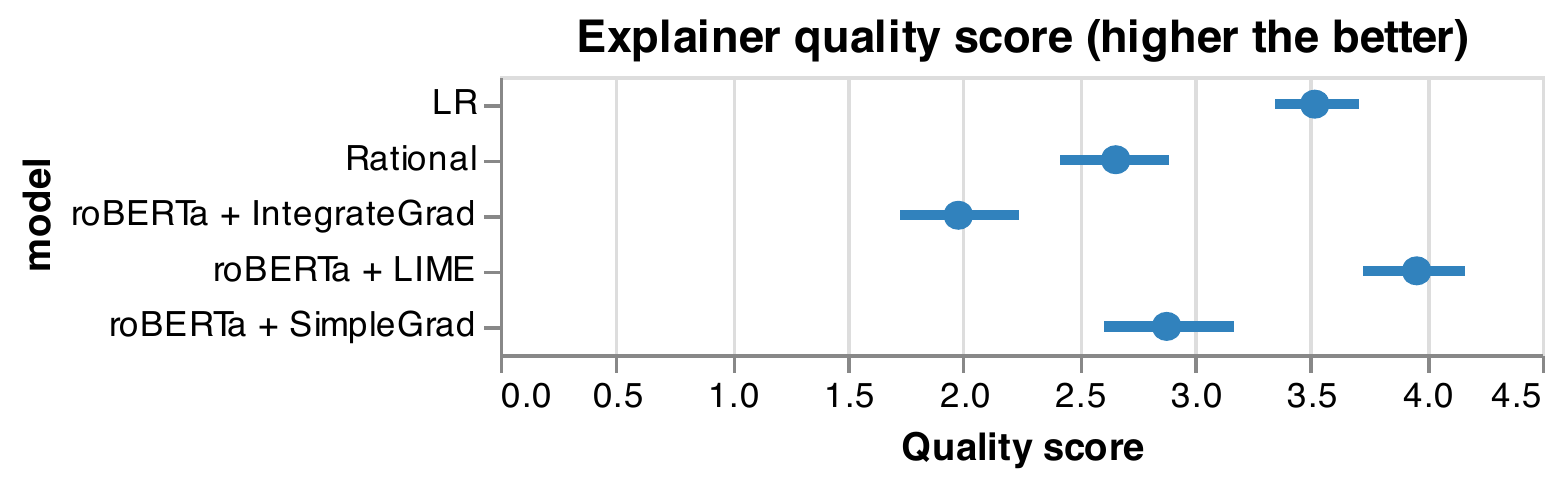}
 \caption{Among the many approaches we tried, roBERTA+LIME was consistently ranked higher than others. \textbf{roBERTa+LIME} appeared to be most highly scored ($3.96 \pm 1.2$).}
 \label{fig:explainer_score}
\end{figure}

% \paragraph{Procedure}
We conducted the following small study on \dbeer to select a model for both datasets: We selected ten beer reviews (five positive and negative) on which all three models were correct and analyzed explanations for the predicted class (highlighted similar to our main task). Since we experimented with three explainers for RoBERTa, we analyzed five explanations per example.
% We anonymized these explanations by removing the system names and randomizing their ordering.
Then, we asked ten graduate students in computer science to rank the explainers from the best quality (score 5) to the worst (score 1). Specifically, we asked them to {\em ``rank the explainers by quality, \ie, which explainer picks the most reasonable words associated with predicted positive/negative sentiment.''} All explanations were anonymized and randomly ordered.
\begin{comment}
%%%% instruction
Please help judge the quality of five explainers on sentiment analysis models!
Explainers highlight the most important words for a model’s prediction.
The explainer will highlight spans of text in red when they make the model think Negative Sentiment is the right choice (similarly blue for Positive)

You will see the outputs of the five explainers (labeled a,b,c,d,e) on 10 beer reviews (5 positive and 5 negative; The models correctly predict all of the sentiments.)
The order of the explainers are randomized.

Your task is to order the explainers by quality (\ie, which explainer picks the most 
reasonable words associated with the corresponding positive/negative sentiment?)

Please order the explainers by quality (e.g., abcde if you think a is the best explainer), and send your result to Sherry in the following format:
\end{comment}

For our main task, we selected the setting that received the highest average score across participants and reviews, which was \emph{roBERTa+LIME} (Figure~\ref{fig:explainer_score}).

\subsection{Stratified Sampling Using Classifier's Confidence}
\label{subsec:confidence_sample}
% \mbox{}\\
Despite performing calibration, our \emph{roBERTa} model produced a highly skewed distribution of confidence scores (Figure~\ref{fig:explainer_score}A). For example, a large number of test examples had a confidence score greater than 0.99, which is problematic for our studies. If all (or most) samples have a confidence score greater than 0.99, then showing confidence scores to users is essentially uninformative.
Since a uniformly randomly drawn study sample would inherit a similar skew, we performed stratified sampling.

\begin{figure}
 \centering
 \includegraphics[width=1\columnwidth]{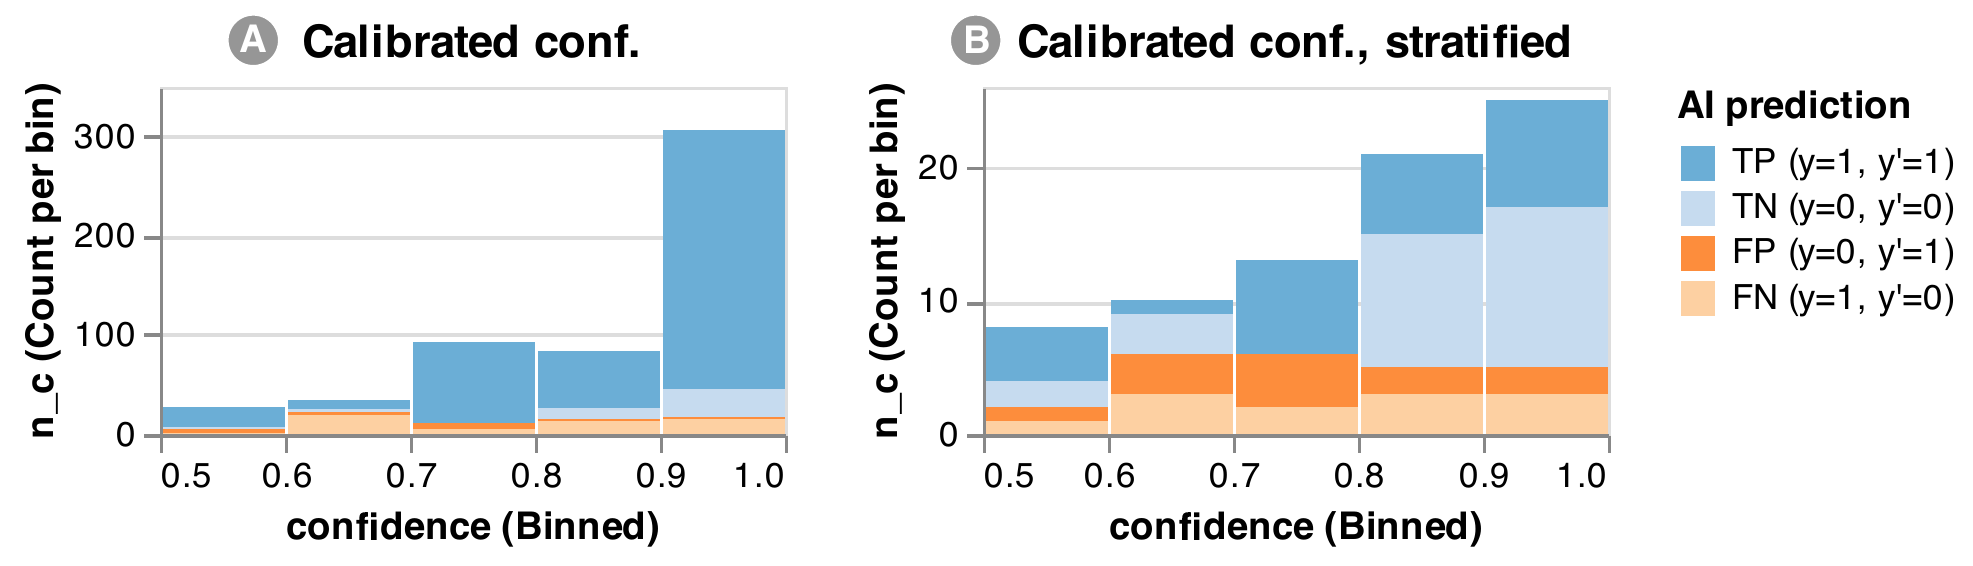}
 \caption{A comparison of the confidence distribution, before and after stratified sampling. The sampling helped select examples to achieve a controlled confidence distribution needed for our analysis.}
 \label{fig:confidence_sample}
\end{figure}

To select examples with a wide range of confidence scores, we first sampled examples such that 0.5 $\leq$ confidence $<$ 0.99, and binned them with a step size of 0.1~(Figure~\ref{fig:confidence_sample}A).
We then performed stratified sampling to draw examples from sub-populations defined by a confidence bin and category of AI prediction: True Positive, True Negative, False Positive, and False Negative.
Since drawing equal number of samples for each sub-population may be too unnatural, for each confidence bin in a prediction category, we drew samples proportional to the logarithmic of number of samples in that bin.
Let $n_{c, p}$ denote number of samples in confidence bin $c$ with prediction category $p$. We drew $m_{c, p}$ samples such that:

\begin{equation*}
 m_{c, p} = \frac{\ln(n_{c, p})}{\sum_{c'}(\ln(n_{c', p}))} \cdot n_{*, p}
\end{equation*}

As shown in Figure~\ref{fig:confidence_sample}A, our sampling helped to construct a subset with a reasonable number of examples per bin, with different AI predictions.
